# Supplementary material for: Protecting GNSS-based Services using Time Offset Validation
Source: arXiv:2202.10891 source file (2022-02-22)
Supplement: Supplementary file 1 [file appendix.tex]

\section{Appendix}
\label{sec:appendix}

%\afterpage{
%	\clearpage
%	\thispagestyle{empty}
	\begin{landscape}
		\begin{table}
			\centering
			\caption{Technology candidates and synthetic evaluation of performances. The candidates are listed by connectivity type, limitations and advantages are presented, alongside the expected accuracy.}
			\label{tab:tech-table}
			\begin{tabular}{|p{4cm}|p{4cm}|p{4cm}|p{4cm}|p{4cm}|}
				\hline
				\rowcolor{gray}
				Technology & Availability & Timing & Accuracy & Vulnerability \\
				\hline
				Cellular 2G, 3G, 4G (connectionless) & Available depending on the generation (Urban areas 4G, more rural areas 2/3G) & TA frames can be used to know the clock difference with the base station & Accuracy is limited to the accuracy of TA: level of \SI{}{\micro\second}. UE needs to be able to process TA from  multiple base stations. & Vulnerable to spoofing attack if the cellular cell equiped with a GNSS receiver is within the range of the GNSS spoofer. \\
				\hline
				Cellular 2G, 3G, 4G (connected) & Available depending on the generation (Urban areas 4G, more rural areas 2/3G) & NTP services running over cellular link can provide timing information. But challenges are due to the sleeping mode of the cellular radio, especially in power constrained systems. & NTP accuracy over LTE is limited to 10ms in case the radio never enters sleep state. Performance degrades when the radio is allowed to idle. SIB16 + TA enhanced SCS has reference granularity of 250ns. &  Vulnerable to spoofing attack if the cellular cell equiped with a GNSS receiver is within the range of the GNSS spoofer.\\
				\hline
				5G & Experimental cellular deployments & URLLC services provide ultra reliable low latency links & Limited infrastructure availability. & Vulnerable to spoofing attack if the cellular cell equiped with a GNSS receiver is within the range of the GNSS spoofer.\\
				\hline
				WLAN (WiFi) & Requiring dedicated radios, but they are common on many platforms. Infrastructure is largely available in urban areas. & Beacon frames contain timestamps with \SI{}{\micro\second} accuracy, which can be used to verify GNSS time stamps across multiple APs. & Beacons emit at rate of 100ms. In crowded wifi environments, interleaving of beacon transmissions can be leveraged to reduce the detection window. & Malicious beacons can be used to manipulate the verification. \\
				\hline
				LoRa (and other 802.15.4 enabled networks) & Requires dedicated radio, which is not common on many platforms. & Beacons based synchronization, with dedicated algorithms like RBS, obtain high synchronization between sensors. & Level of \SI{}{\micro\second} accuracy is achievable & Malicious beacons can be used to manipulate the verification. \\
				\hline
				Local oscillators & Available on each MCU based system, with different features available for different architectures and designs. & Provide very accurate timing information. TSC (time stamp counter) in x86 architectures can be used to evaluate the time by measuring instructions execution. & High stability clock sources are available in state-of-art processors, as good as \SI{0.1}{PPM} and TSC registers allow access to raw clock information from CPU to detect variation of the spoofed GNSS time. & Sensitive to environmental changes, e.g., temperature and voltage.  \\
				\hline
			\end{tabular}
			
		\end{table}
	\end{landscape}
%	\clearpage
%} 
